# Supplementary material for: Predicting Political Ideology from Digital Footprints
Source: arXiv:2206.00397 source file (2022-06-01)
Supplement: Supplementary file 1 [file AppendixA.tex]

\chapter{Scripts}
\label{Appendix-scripts}

This appendix outlines the psuedo code for the user flair scraper, user history scraper, data manipulator, comment scraper and comment manipulator scripts.
