# Supplementary material for: Predicting Political Ideology from Digital Footprints
Source: arXiv:2206.00397 source file (2022-06-01)
Supplement: Supplementary file 2 [file AppendixC.tex]

\chapter{Model details}
\label{Appendix-Models}

Here we report the

Specific details of all models used
