# Supplementary material for: Predicting Political Ideology from Digital Footprints
Source: arXiv:2206.00397 source file (2022-06-01)
Supplement: Supplementary file 6 [file AppendixRemoved.tex]

\chapter{Subreddits removed}
\label{Appendix-removed}

We removed the following subreddits from our user-interaction matrix:

\begin{itemize}
    \item r/Libertarian
    \item r/Anarchism
    \item r/socialism
    \item r/progressive
    \item r/Conservative
    \item r/democrats
    \item r/Liberal
    \item r/Republican
    \item r/Liberty
    \item r/Labour
    \item r/Marxism
    \item r/Capitalism
    \item r/Anarchist
    \item r/republicans
    \item r/conservatives 
\end{itemize}
